# Supplementary material for: Online Marketplace: A Benchmark for Data Management in Microservices
Source: arXiv:2403.12605 source file (2025-01-11)
Supplement: Supplementary file 1 [file 99_appendix.tex]

\section{Appendix}

The appendix contains further details about \OM\ benchmark specification, including the data model ($\S$~\ref{subsec:data_model}), the event schema~\ref{subsec:event_schema}, the remaining specification of the continuous queries from $\S$~\ref{subsec:queries} ($\S$~\ref{subsec:extended_queries}), the required APIs ($\S$~\ref{apx:apis}), the driver's workload manager ($\S$~\ref{apx:driver}), the design of the components ($\S$~\ref{apx:design}), and additional Statefun configuration ($\S$~\ref{apx:statefun}). %, and a suggested implementation of the business logic of the prescribed microservices ($\S$~\ref{subsec:impl}). 

\subsection{Data Model}
\label{subsec:data_model}

Figure~\ref{fig:data_model_microservices} shows the complete data model of \OM\ microservices.

\begin{figure*}
\centering
  \includesvg[width=1\textwidth]
  {figures/draft_model_1.svg}
  \vspace{-3ex}
\caption{\OM\ Data Model}
\label{fig:data_model_microservices}
\vspace{-2ex}
\end{figure*}

\subsection{Event Schema}
\label{subsec:event_schema}

Table~\ref{tab:event_schema} shows the event schema of \OM\ microservices. % Users can refer to one of the implementations to get specific event schemas for data platforms, due to programming modelsdifference, event schemas canvary. refer to ...
% \textcolor{red}{put events in some defined structure with types, like avro or graphql}

% schema: type and name of the field

\begin{table*}
\centering
\caption{Events Processed by \OM}
\vspace{-3ex}
\begin{tabularx}{\linewidth}{SYcSS}
\toprule
\textbf{Event Type} & \textbf{Event Schema} & \textbf{Producer} & \textbf{Consumers} & \textbf{Transaction} \\
\hline
% \texttt{addItem\_cart} & \texttt{} & Driver & Cart & Customer Checkout \\
% \hline
% \texttt{checkout\_cart} & \texttt{customer\_id, discounts, items} & Cart & Order & Customer Checkout \\
% \hline
\texttt{Price Update} & \texttt{seller\_id, product\_id, newPrice, version} & Product & Cart & Update Price \\
\hline
\texttt{Product Delete} & \texttt{seller\_id, product\_id, version} & Product & Stock & Delete Product \\
\hline
\texttt{Reserve Inventory} & \texttt{ checkout\_info \{customer\_id, payment\_type, card\_number, ... \}, items: [\{seller\_id, product\_id, price, version\}, ... ], timestamp} & Cart & Stock & Customer Checkout \\
\hline
\texttt{Stock Confirmed} & Same as \texttt{Reserve Inventory} & Stock & Order & Customer Checkout \\
\hline
\texttt{Stock Reservation Failed} & Same as \texttt{Reserve Inventory} & Stock & Customer & Customer Checkout \\
\hline
\texttt{Invoice Issued} & \texttt{order\_id, invoice\_num, total\_amount, customer\_info \{customer\_id, payment\_type, card\_number, ... \}, items: [\{seller\_id, product\_id, price, version\}, ... ], timestamp} & Order & Payment, Seller & Customer Checkout \\
\hline
\texttt{Payment Confirmed} & Same as \texttt{InvoiceIssued} & Payment & Order, Seller, Shipment & Customer Checkout \\
\hline
\texttt{Payment Failed} & Same as \texttt{InvoiceIssued}, but including status & Payment & Order, Seller & Product Update \\
\hline
\texttt{Shipment Notification} & \texttt{order\_id, invoice\_num, shipment\_id, shipment\_status, timestamp} & Shipment & Order, Seller & Customer Checkout \& Update Delivery \\
\hline
\texttt{Delivery Notification} & \texttt{order\_id, invoice\_num, shipment\_id, package\_id, seller\_id, product\_id, delivery\_status, timestamp} & Shipment & Seller, Customer & Update Delivery \\
\hline
\end{tabularx}
\label{tab:event_schema}
\vspace{-1ex}
\end{table*}

\subsection{Continuous Queries}
\label{subsec:extended_queries}

In this section, we specify the remaining continuous queries presented in Section~\ref{subsec:queries}.

\subsubsection{Cart Abandonment}
\label{apx:cart}

Assuming there is a stream that is the union of both failed payments and failed reservations,
one could implement \textbf{Cart Abandonment} in ksql~\cite{kafka_streams} through the following continuous query:

% stream 1:
% create stream failed_payments as
% select cartid, "payment" as type
% from 
% \texttt{payment_result} where status = failed
% emit changes;

% stream 2:
% create stream failed_reservation as
% select cartid, "reservation" as type
% from 
% \texttt{reservation_result} where status = failed
% emit changes;

% create stream failed_checkouts as
% select cart id and ts
% from \texttt{checkout_cart} as c
% left Join failed_reservation
% left failed_payment
% where either must be != null
% emit changes;

\begin{lstlisting}[language=SQL]
create stream failed_checkouts as
select cart id and ts
from checkout_cart as c
inner join failed_events on cartid

select failed_checkouts.cartid 
from failed_checkouts as fc
left join checkout_cart as c
within 10 minutes ON stream1.cartid = stream2.cartid and stream2.ts > stream1.ts
where stream2.cartid is null
emit changes;
\end{lstlisting}

% event with the union of two streams: (i) \texttt{reservation_result} where status = "FAILED" and (ii) \texttt{payment_result} where status = "FAILED".
% the criteria for joining is the \textit{cart_id}.
% EMIT CHANGES;

% on ksql, define on producer the timestamp of each stream so the ksql make the join window work

% To match, there must be a difference of time (e.g., a day. 10 minutes, etc) between the LAST \texttt{checkout_cart} event and the correspondents, in addition to the matching criteria (attribute \texttt{cart_id} in both events). If a match is found, an event is generated to the stream of \textit{abandoned_carts}. those which have not been resubmitted.

% checkout d1, OR(out-of-stock,failed-payment), NO NEW checkout in d2
% WINDOW 10 min
% ---> generate abandoned-cart event

% Should trigger an email to remember customer.
% However, only once. If the user logs again and do nothing, the cart and order must be abandoned.

% https://materialize.com/customer-stories/drizly/

% \begin{lstlisting}[caption={blabla,language=rock,numbers=none,label={lst:abandoned},captionpos=b]]
% \end{lstlisting}

\subsubsection{Low Stock Warning}
\label{apx:stock}

The continuous query to warn sellers about low stock can be specified through the following statements in ksql:
% resident stock state
% build table in memory with starting stock
% create stream stock_decrement
% based on the event payment success,
% that tells us the stock sold
% to decrement from the memory_stock_table
% # create stream stock_increment to listen from the event stock_replenishment
% that tells us the stock replenished
% to increment to the memory_stock_table
\begin{lstlisting}[language=SQL]
create stream qty_orders_per_week
select productid, ts, sum(quantity) as sum
from checkout_item as c
group by productid
sliding window 1 week

create stream agg_checkout
select productid, sum(quantity)/count(*) as avg
from qty_orders_per_week as q
group by productid
sliding window 1 month

create stream stockthreshold
select productid, avg
from agg_checkout as c
inner join memory_stock_table as mem on productid
where mem.quantity < avg
emit changes;
\end{lstlisting}

% aggregate of last week
% if stock is lower, we generate the low stock event
% create stream of aggregate
% and then the low one

% \newpage

\subsection{Required APIs}
\label{apx:apis}

Table~\ref{tab:apis} show the APIs required in order to allow the driver to interact with microservices.

\begin{table*}
\centering
\caption{Required HTTP APIs}
\vspace{-3ex}
\begin{tabular}{cccc}
\toprule
\textbf{API} &
  \textbf{HTTP Request Type} &
  \textbf{Microservice} &
  \textbf{Description} \\
  \hline
/cart/\{customerId\}/add      & PUT   & Cart     & Add a product to a customer's cart    \\
\hline
/cart/\{customerId\}/checkout & POST  & Cart     & Checkout a cart                       \\
\hline
/cart/\{customerId\}/seal     & POST  & Cart     & Reset a cart                          \\
\hline
/customer                     & POST  & Customer & Register a new customer               \\
\hline
/product                      & POST  & Product  & Register a new product                \\
\hline
/product                      & PATCH & Product  & Update a product's price              \\
\hline
/product                      & PUT   & Product  & Replace a product                     \\
\hline
/seller                       & POST  & Seller   & Register a new seller                 \\
\hline
/seller/dashboard/\{sellerId\} &
  GET &
  Seller &
  Retrieve seller's dashboard for a given a seller \\
  \hline
/shipment/\{tid\}             & PATCH & Shipment & Update packages to 'delivered' status \\
\hline
/stock                        & POST  & Stock    & Register a new stock item \\
\hline
\end{tabular}
\label{tab:apis}
\end{table*}

\subsection{Driver Architecture}
\label{apx:driver}

The driver's workload manager is exhibited in Figure~\ref{fig:workload_manager}. The workload manager ensures transactions are submitted within a time frame specified by the user. Besides, the driver controls the maximum number of concurrent transactions running in the target platform by (i) Initializing a number of threads defined by the concurrency level. Each thread simulates a user interacting with the application; (ii) Whenever a transaction result returns, the driver pulls a previously used thread from a thread pool and spawns a new transaction submission.

\begin{figure*}
\centering
  \includesvg[width=0.7\textwidth]
  {figures/workload_manager.svg}
  \vspace{-3ex}
\caption{Driver Workload Manager}
\label{fig:workload_manager}
\vspace{-1ex}
\end{figure*}

\subsection{Components Design}
\label{apx:design}

Table~\ref{tab:components_design} exhibits the components' design of both actors and functions in Orleans and Statefun, respectively.

\begin{table*}
\caption{Components Design}
% \vspace{-3ex}
% \begin{tabularx}{\columnwidth}{cY}
\begin{tabular}{cc}
 \hline
 Actor/Function & Description \\
 \hline
Cart & Models a customer's cart state and behavior \\ 
 \hline
 Customer & Models a customer's state and behavior \\
 \hline
 Seller & Models a seller's state and behavior \\
 \hline
 Product & Models a product's state and behavior \\
 \hline
  Stock & Models a stock item's state and behavior \\
 \hline
  Order & Models a unit of order processing for a single customer and associated state \\
 \hline
  Payment & Models a unit of payment processing for a single customer \\
 \hline
 Shipment & Models a unit of shipment processing for a disjoint group of customers and related state \\
 \hline
% \end{tabularx}
\end{tabular}
% \vspace{-1ex}
\label{tab:components_design}
% \vspace{-3ex}
\end{table*}

\subsection{Statefun Configuration}
\label{apx:statefun}

We followed Flink's memory tuning~\footnote{https://nightlies.apache.org/flink/flink-docs-release-1.18/docs/deployment/memory/mem\_tuning} and configuration\footnote{https://nightlies.apache.org/flink/flink-docs-release-1.18/docs/deployment/config/} guidelines in order to configure Statefun instance for our experiments. The configuration used is shown in Listing~\ref{lst:statefun}.

\begin{lstlisting}[caption={Statefun Configuration},label={lst:statefun},captionpos=b]
state.backend=hashmap 
jobmanager.memory.process.size=24 gb
taskmanager.memory.process.size=24 gb
taskmanager.memory.managed.size=0 gb
taskmanager.numberOfTaskSlots=6
parallelism.default=6
statefun.async.max-per-task=16000
maxNumBatchRequests: 15
\end{lstlisting}
